# Supplementary material for: BaB-ND: Long-Horizon Motion Planning with Branch-and-Bound and Neural Dynamics
Source: arXiv:2412.09584 source file (2025-03-16)
Supplement: Supplementary file 1 [file fig_real.pdf]

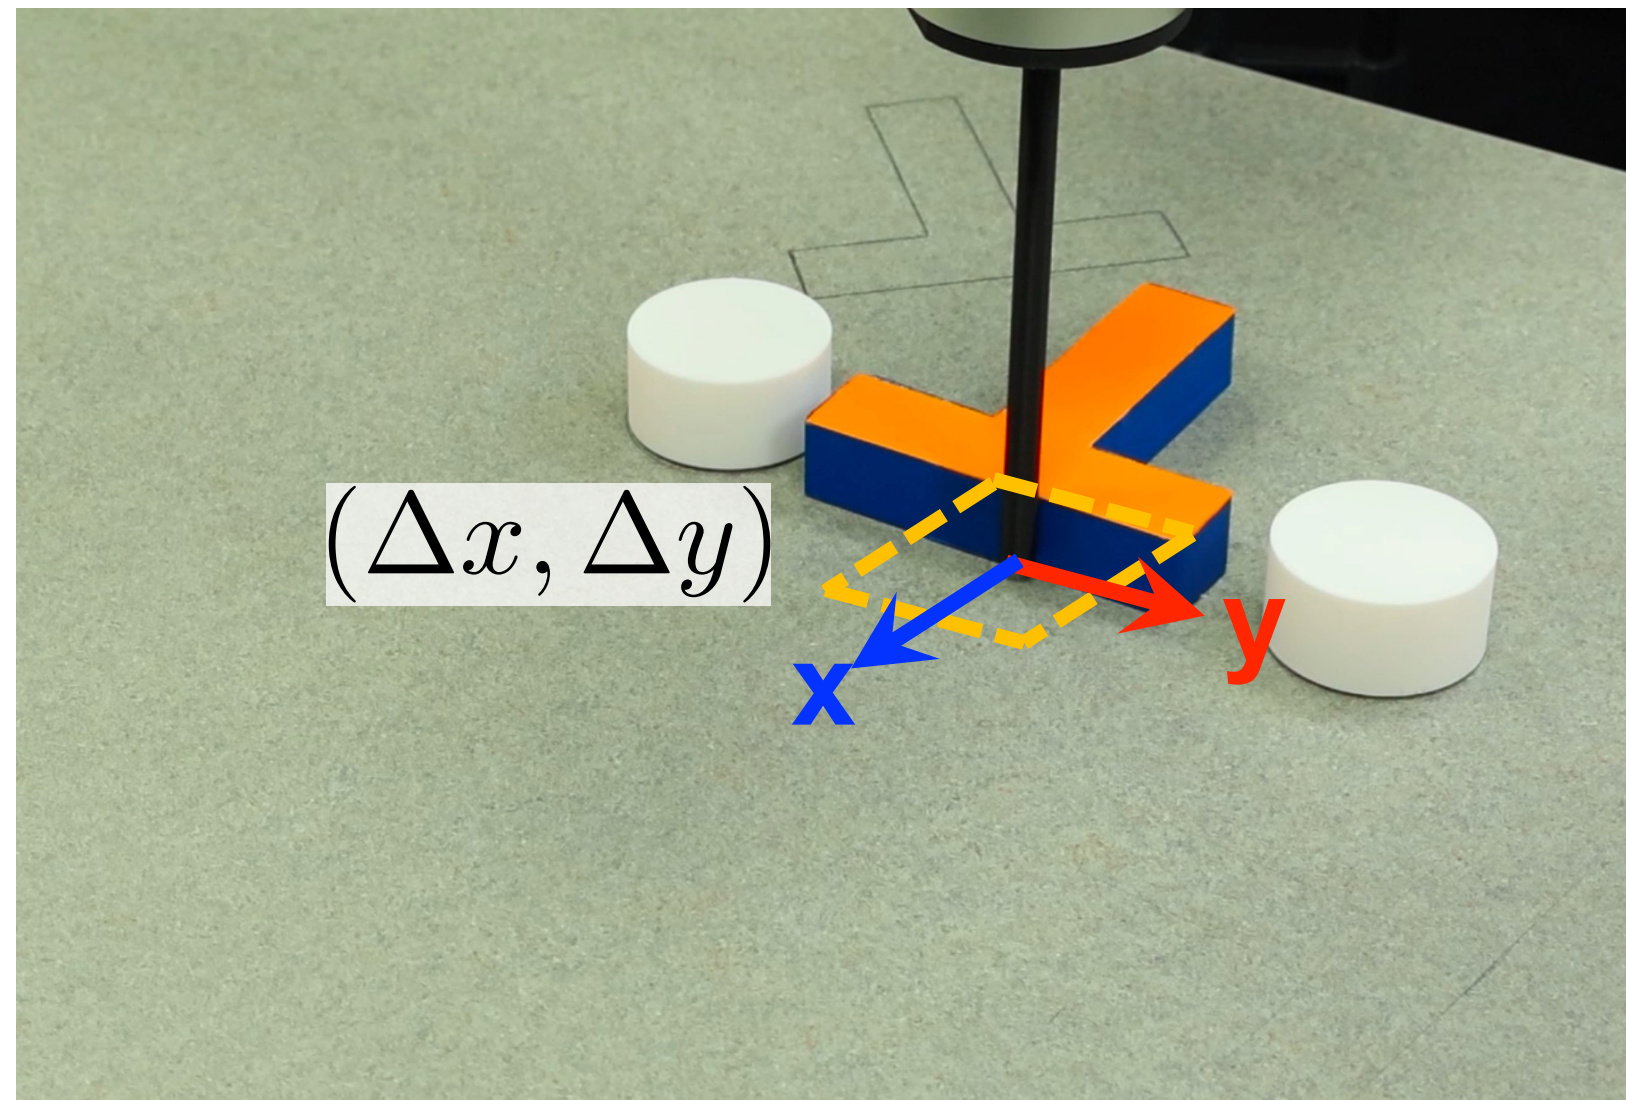

(a) Pushing w/ Obstacles

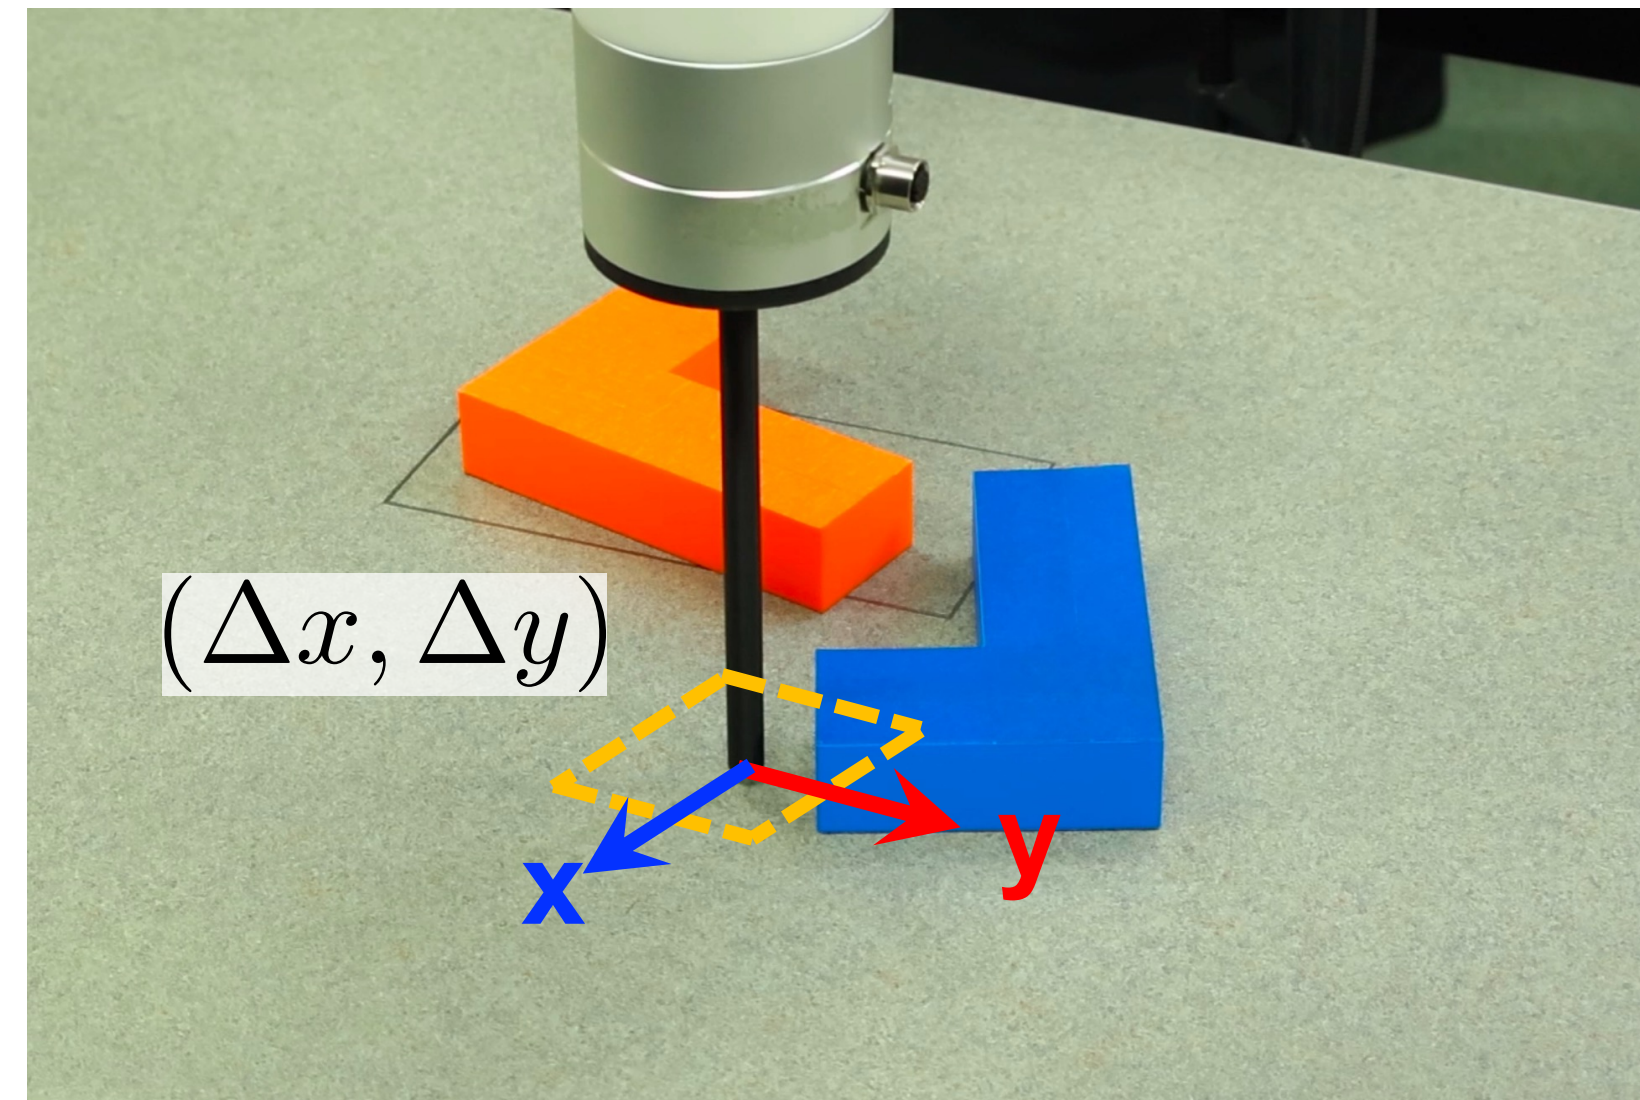

(b) Object Merging

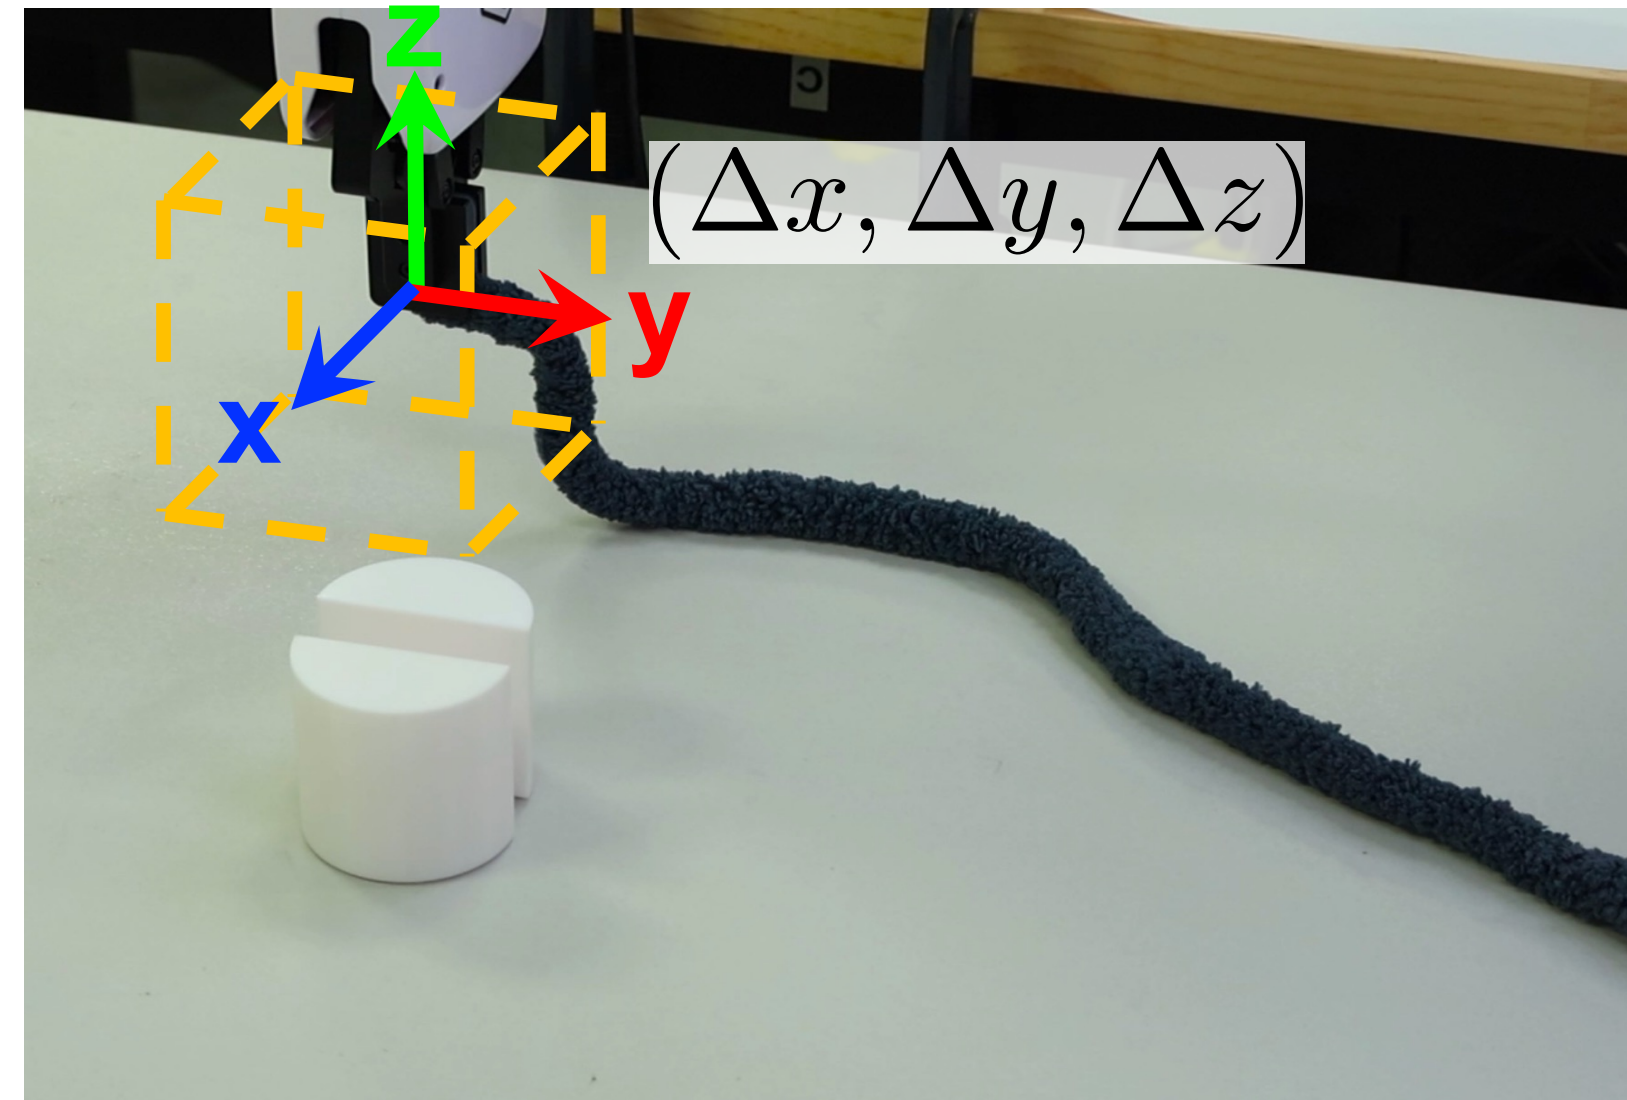

(c) Rope Routing

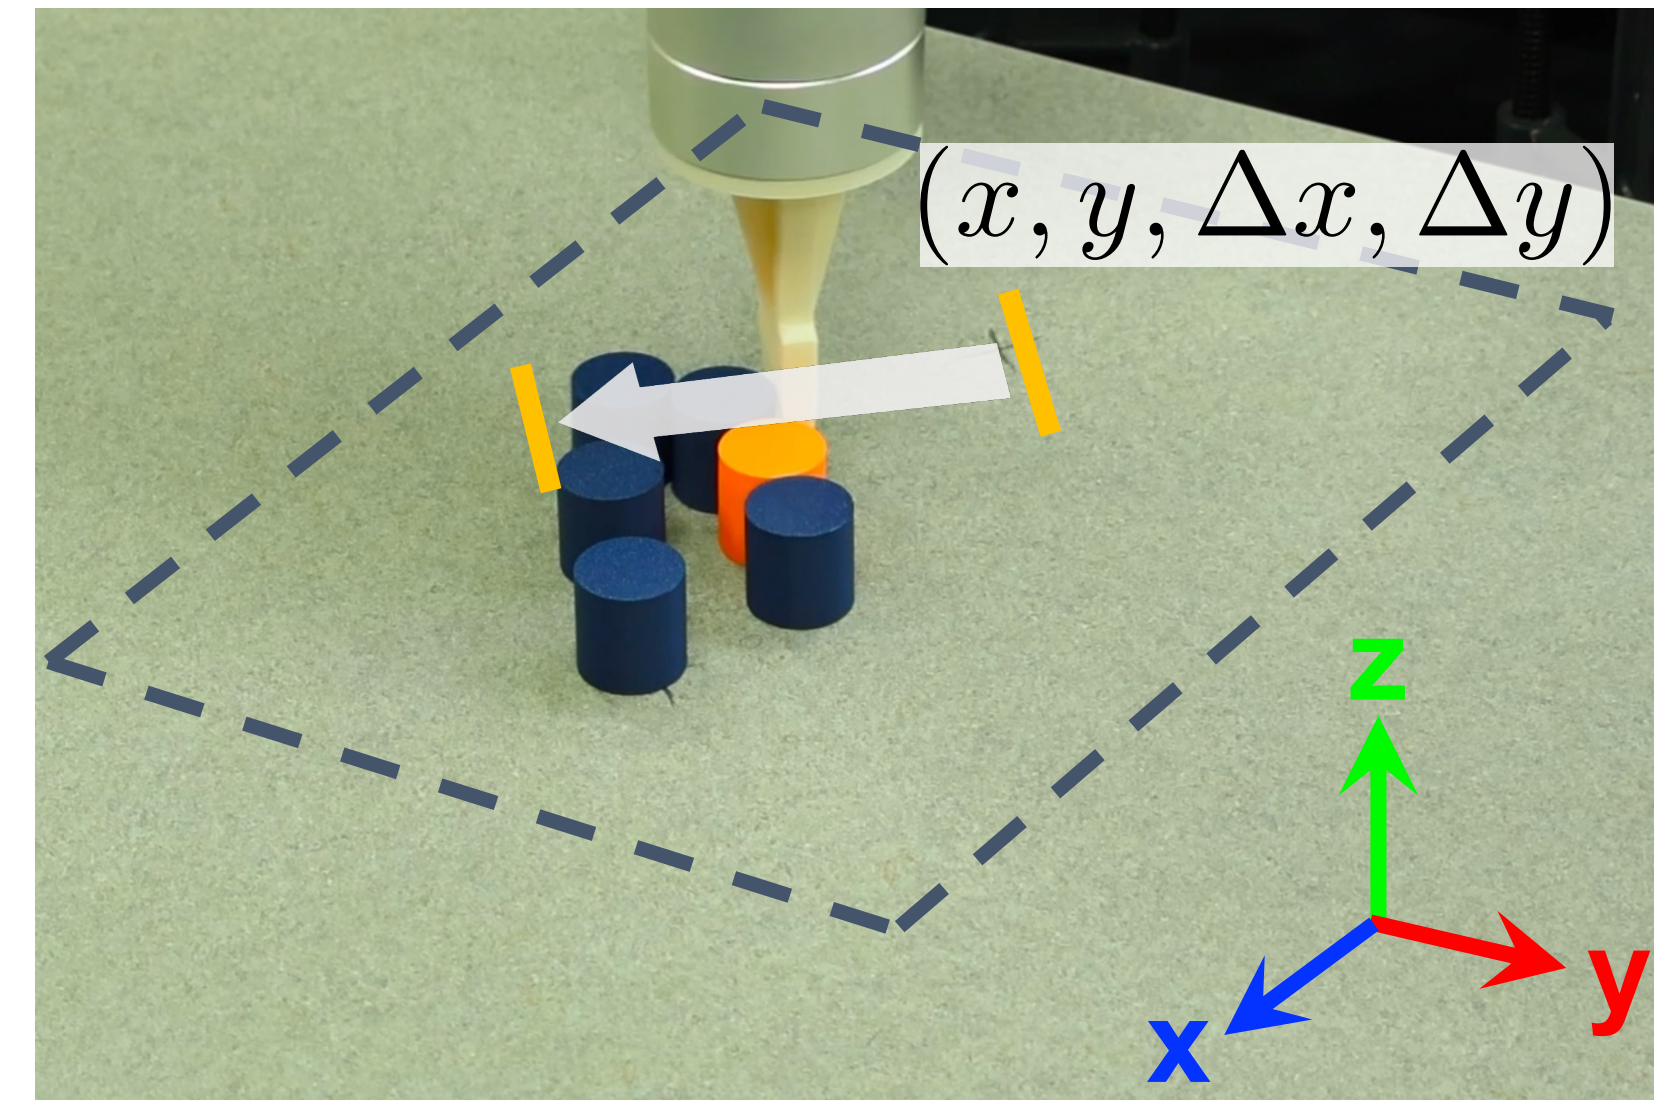

(d) Object Sorting



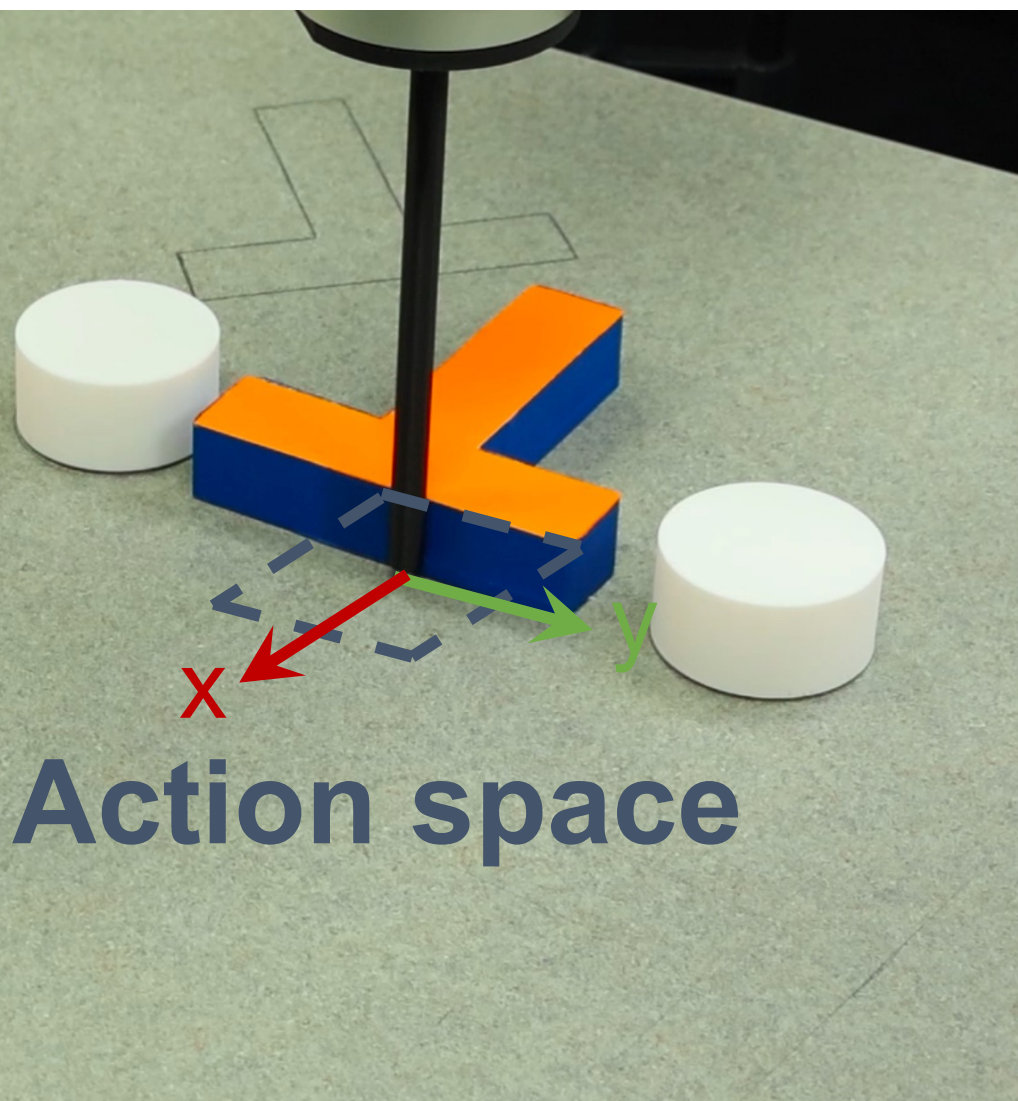

ing w/ Obstacles

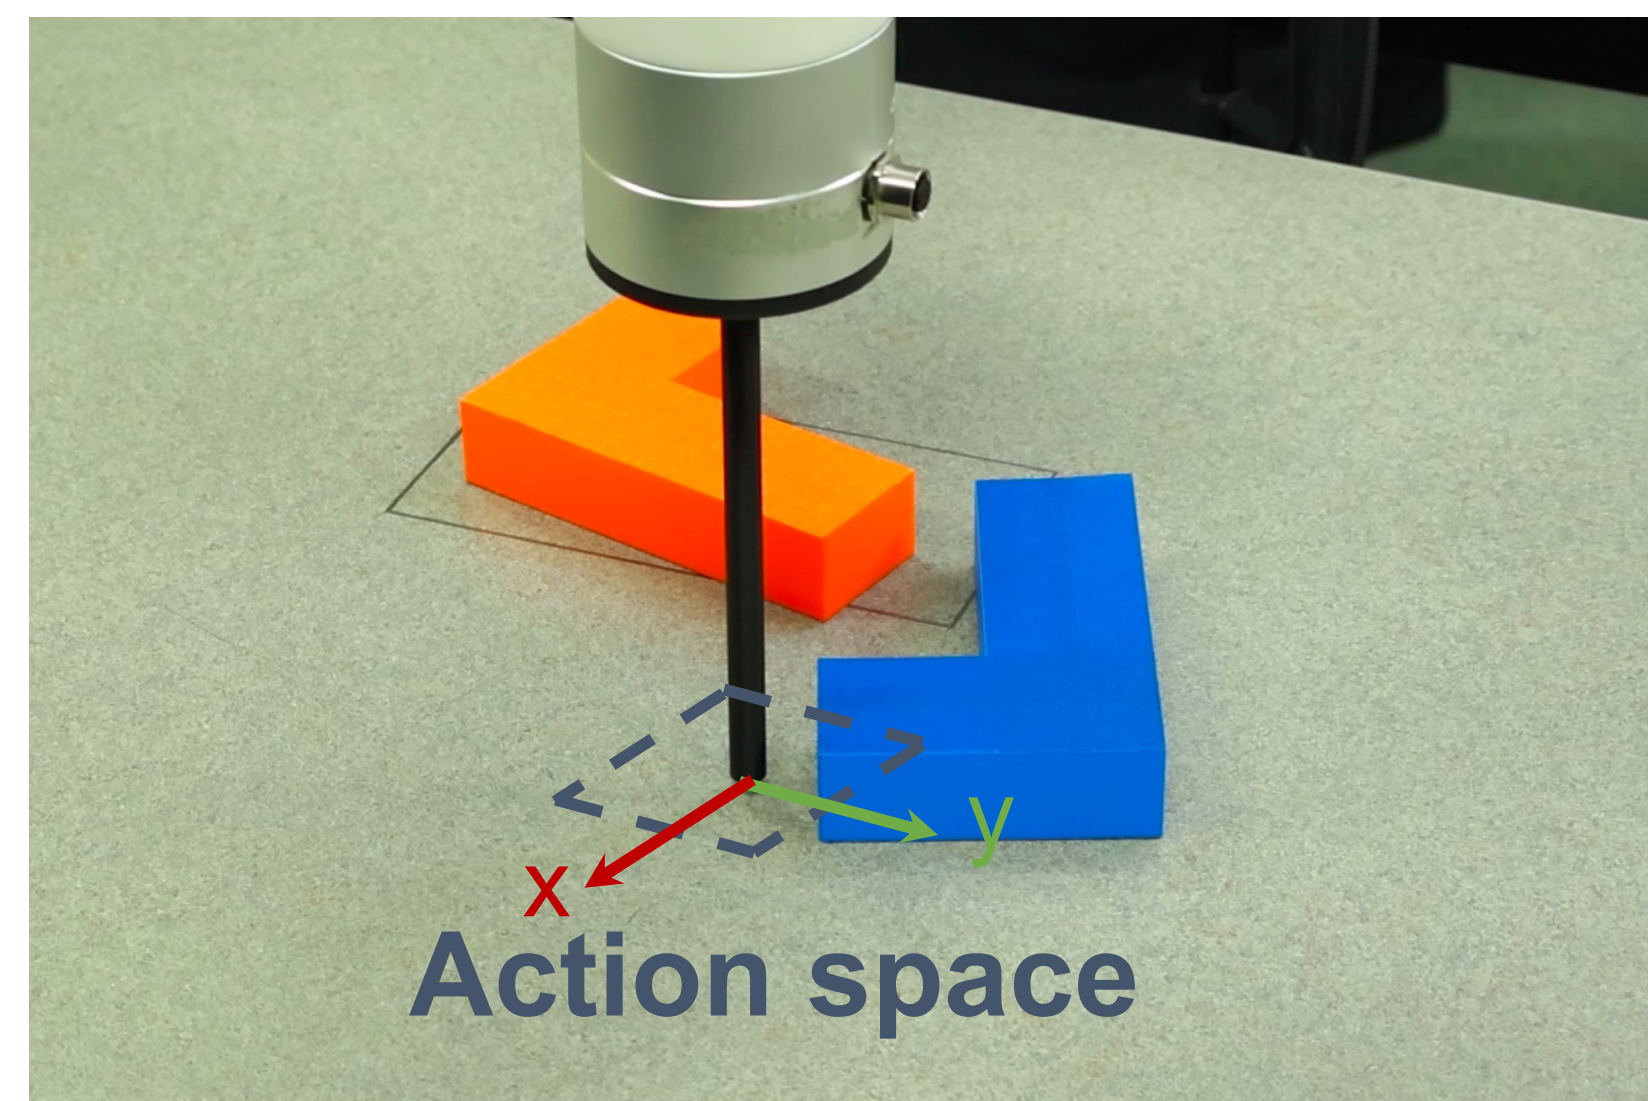

(b) Object Merging

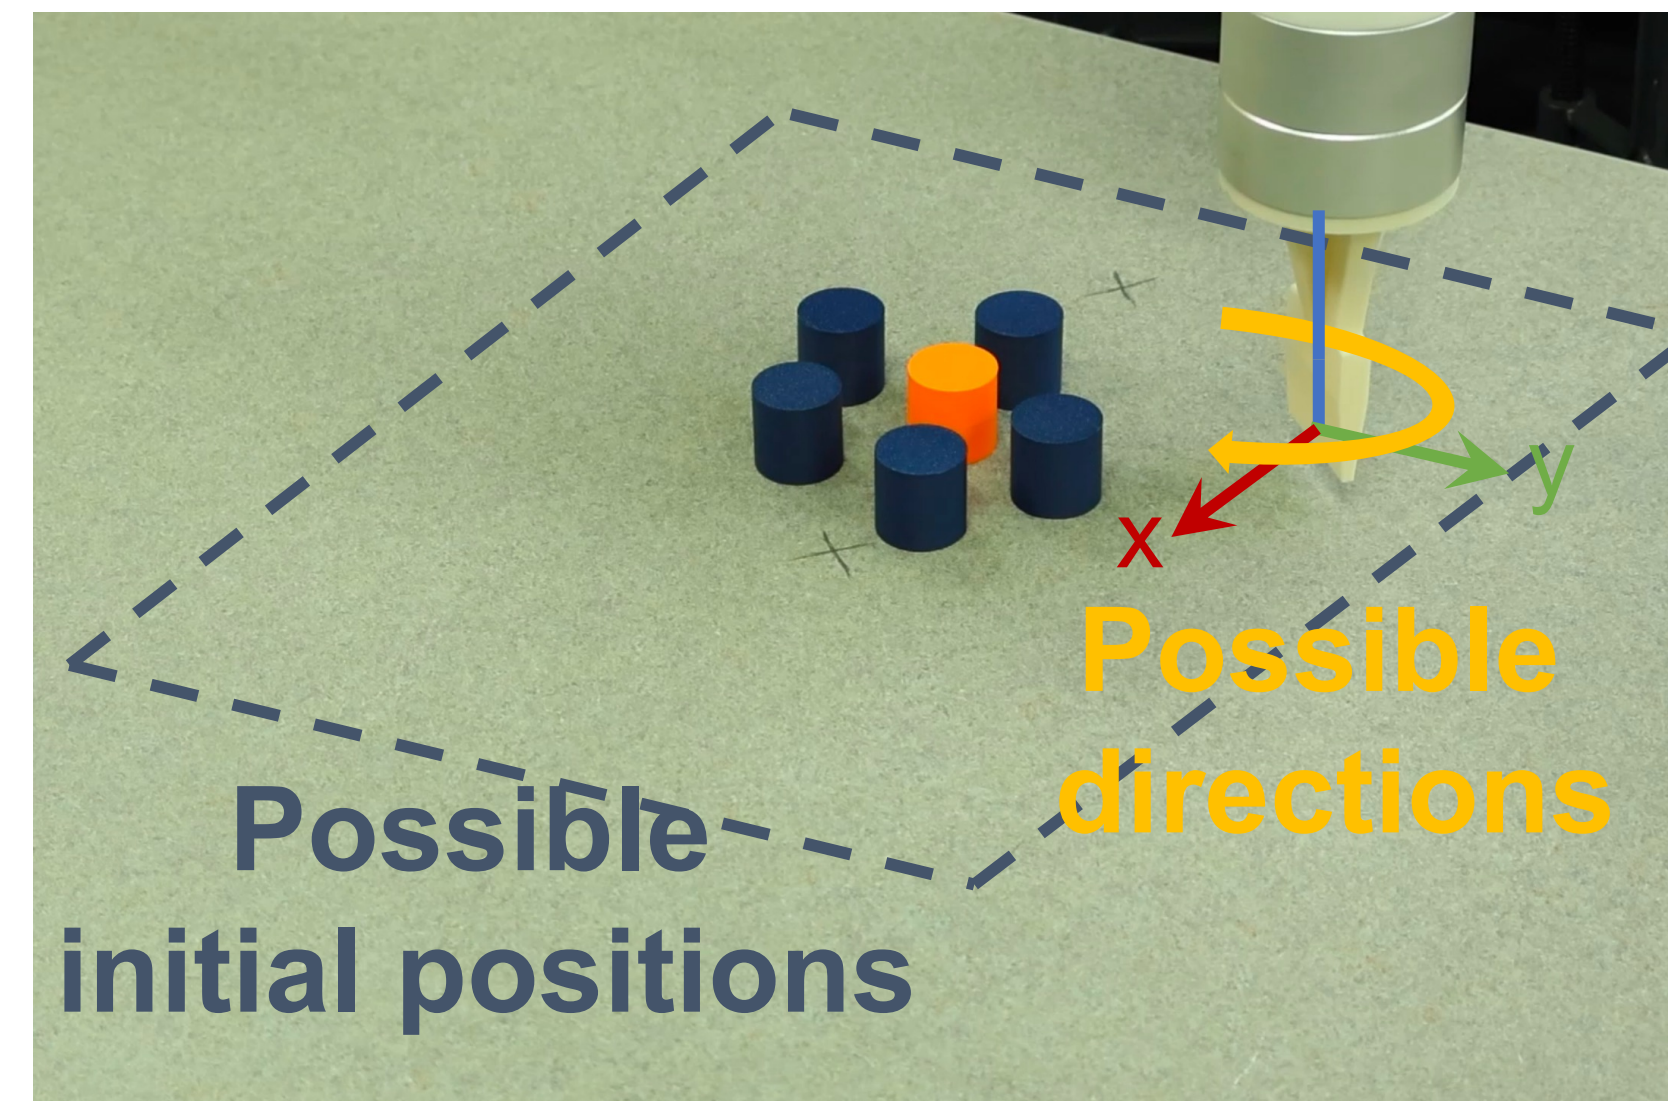

(c) Object Sorting

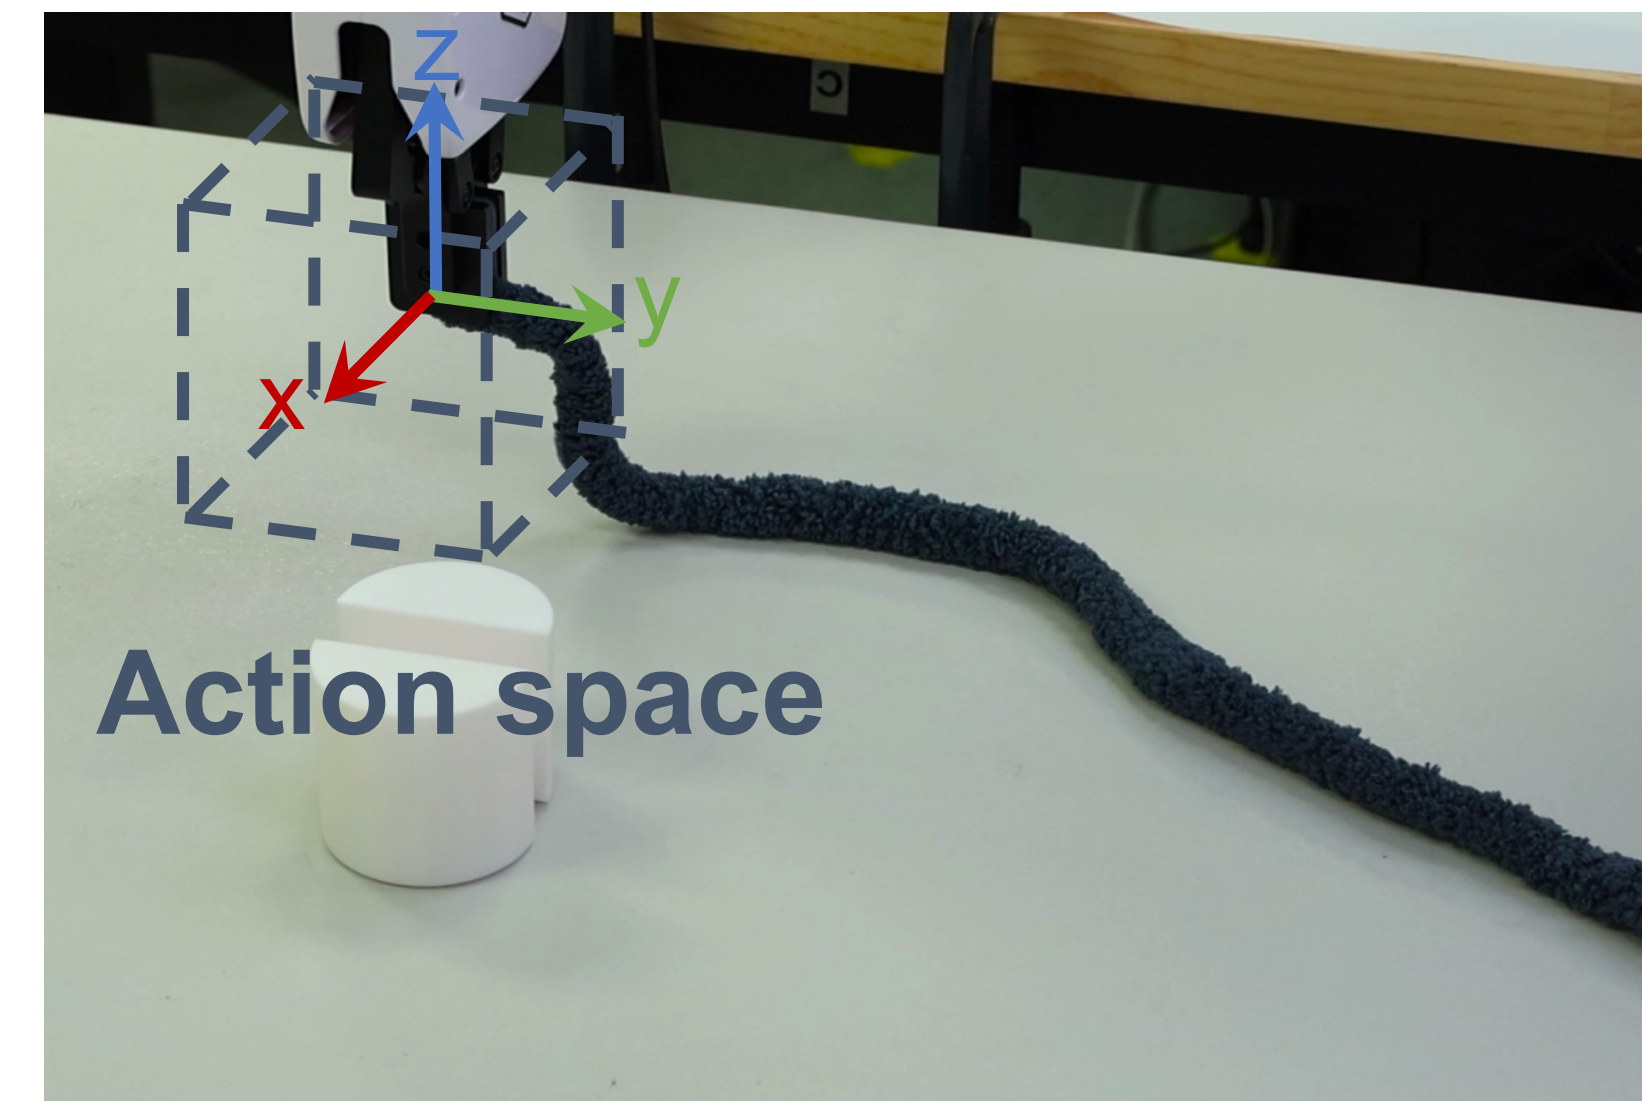

(d) Rope Routing
